# Supplementary material for: DASP: A Framework for Driving the Adoption of Software Security Practices
Source: arXiv:2205.12388 source file (2022-05-24)
Supplement: Supplementary file 1 [file appendix.tex]

\appendices
\section{Proof of the First Zonklar Equation}
Appendix one text goes here.

% you can choose not to have a title for an appendix
% if you want by leaving the argument blank
\section{}
Appendix two text goes here.

\vspace{5px}
